# Supplementary material for: Communication-Efficient MARL for Platoon Stability and Energy-efficiency Co-optimization in Cooperative Adaptive Cruise Control of CAVs
Source: arXiv:2406.11653 source file (2024-06-17)
Supplement: Supplementary file 1 [file Appendix.tex]

% \documentclass[lettersize,journal]{IEEEtran}
% \usepackage{graphicx} % For \includegraphics
% \usepackage{subcaption} % For subfigures
% \usepackage{multirow}
% \usepackage{booktabs} % For formal tables
% \usepackage{siunitx} % For unit alignment
% \usepackage{graphicx} % For scaling tables

% \begin{document}
\section{Appendix}
\subsection{Vehicle dynamics and energy consumption}
\subsubsection{\textbf{Longitudinal dynamics}}
The CACC scenario is formulated by a platoon leader vehicle (PL, the $1$st vehicle), followed by the platoon member vehicles (PMs, indexed by $i$ from $2$ to $\mathcal{N}$). Each PM $i$ adheres to a specific spacing policy \cite{hart2024towards} to maintain a pre-determined IVS $d_{i}$ and longitudinal velocity $v_{i}$ with respect to the preceding vehicle ($i-1$). The \textbf{vehicle longitudinal kinematics} for each vehicle $i$ are defined as follows:
\begin{equation}
   \begin{gathered}
\dot{d}_{i}=v_{i-1}-v_{i} \\
\dot{v}_{i}=u_{i}
   \end{gathered}
\label{eq2}
\end{equation}
where $v_{i-1}$ and $u_{i}$ are the longitudinal velocity of its preceding vehicle and the acceleration of vehicle $i$, respectively. Furthermore, the discretized longitudinal kinematics for each vehicle $i$ , given a sampling time $\Delta t$, can be described by
\begin{equation}
   \begin{aligned}
d_{i, t+1}= & l_{i, t}+\int_{t}^{t+\Delta t}\left(v_{i-1, \tau}-v_{i, \tau}\right) d \tau \\
& v_{i, t+1}=v_{i, t}+u_{i, t} \Delta t
\end{aligned}
\label{eq3}
\end{equation}

The driving force of each vehicle, $F_{i}$, can be calculated by
\begin{equation}
\begin{gathered}
F_{i} (t)=mgf\cos \alpha +\frac{1}{2} \rho %A_{f}C_{d}v_{i}^{2}+mg\sin \alpha + mu_{i}\\
P_{i}(t)=F_{i}(t)\cdot v_{i} \\
T_{i}(t)=F_{i}(t)\cdot R
\end{gathered}
\label{eq4}
\end{equation}
where $m$ is the vehicle mass; $g$ is the gravity acceleration; $f$ is the rolling resistance coefficient; $\rho$ is the air density; $A_{f}$ is the front area of the vehicle; $C_{d}$ is the aerodynamic drag coefficient; $R$ is the wheel radius; $\alpha$ is the road slope; in this paper, the road slope is not considered. Table \ref{appendix: table1} lists the critical parameters of the longitudinal dynamics model of the vehicle.

\begin{table}[ht]
    \centering
    \caption{Parameters of Longitudinal Dynamics Model}
    \label{appendix: table1}
    \begin{tabular}{c c}
    \hline\hline
        Description & Value \\
    \hline
        Vehicle mass $m$ & 1718.4 kg \\
        Rolling resistance coefficient $f$ & 0.011 \\
        Air density $\rho$ & 1.206 $\mathrm{kg} / \mathrm{m}^{3}$ \\
        Aerodynamic drag coefficient $C_{d}$ & 0.32 \\
        Frontal area $A_{f}$ & 2.455 $\mathrm{m}^{2}$ \\
        Gravity acceleration $g$  & 9.8 $\mathrm{~m} / \mathrm{s}^{2}$ \\
        Gear ratio $i$ & 3.91 * 4.14 \\
        Wheel radius $R$ & 0.337 m\\
    \hline\hline
    \end{tabular}
\vspace{-10pt}
\end{table}

For simplicity, it's assumed that all vehicles possess the same dynamics and capabilities regarding their energy model and their maximum acceleration and deceleration limits.
To ensure safety, comfort, and power requirements, each vehicle is required to follow the constraints \cite{chu2019model}:
\begin{equation}
   \begin{gathered}
d_{i, t} \geq 1 \mathrm{~m} \\
0 \leq v_{i, t} \leq 30 \mathrm{~m} / \mathrm{s} \\
-2.5 \mathrm{~m} / \mathrm{s}^{2} \leq u_{i, t} \leq 2.5 \mathrm{~m} / \mathrm{s}^{2}
   \end{gathered}
\label{eq5}
\end{equation}

\subsubsection{\textbf{Energy Consumption Model}}
Typically, a polynomial-based, differentiable approximation of an energy consumption model is adequate to create an energy-saving algorithm \cite{10359483}. For the power consumption of the electric motor, the formula for the electric power of each vehicle $P_{i}$ can be calculated as follows:

\begin{equation}
\begin{gathered}
   P_{i} = T_{i} \cdot \omega_{i} \cdot \eta_{i}^{-k} \\
   T_{i}=F_{i}\cdot R 
\end{gathered}
\label{eq}
\end{equation}
where $T_{i}$ represents the motor torque of each vehicle, $\omega_{i}$ is the rotational velocity of the motor for each vehicle, and $\eta_{i}$ is the efficiency of electric-mechanical conversion, detailed in Appendix with Figure \ref{appen2:fig_motor_map}. 
The $k$ indicates the operational mode. $k=1$ denotes the driving model while $k=-1$ denotes regenerative braking mode.  To simplify the calculation and calibration, the vehicle energy consumption, $P_{i}(v_{i}, u_{i})$, is formulated as a function of vehicle velocity $v_{i}$ and acceleration $u_{i}$ as in \cite{guzzella2007vehicle},
\begin{equation}
   P_{i}(v_{i}, u_{i}) = \sum_{k=0}^{4} \sum_{j=0}^{4} p_{kj} \cdot v_{i}^k \cdot u_{i}^j
\end{equation}
where $p_{kj}$ is the polynomial coefficient determined by fitting. We used trial-and-error to identify the polynomial order and coefficients with the Pyhton Fitting Libraries. 
Figure \ref{appen3:fig_power_distribution} and Figure \ref{appen4:fig_residul_power} in Appendix display a contour map showing power consumption relative to vehicle velocity and acceleration, highlighting the 0 kW contour with a red line and a fitting result with residuals mostly near zero and a root mean square error of 0.275 kW respectively.
In this work, each vehicle equipped with the CACC is considered to have identical capabilities and physical characteristics.

\begin{figure}[!ht]
\centerline{\includegraphics[width=1.0\columnwidth]{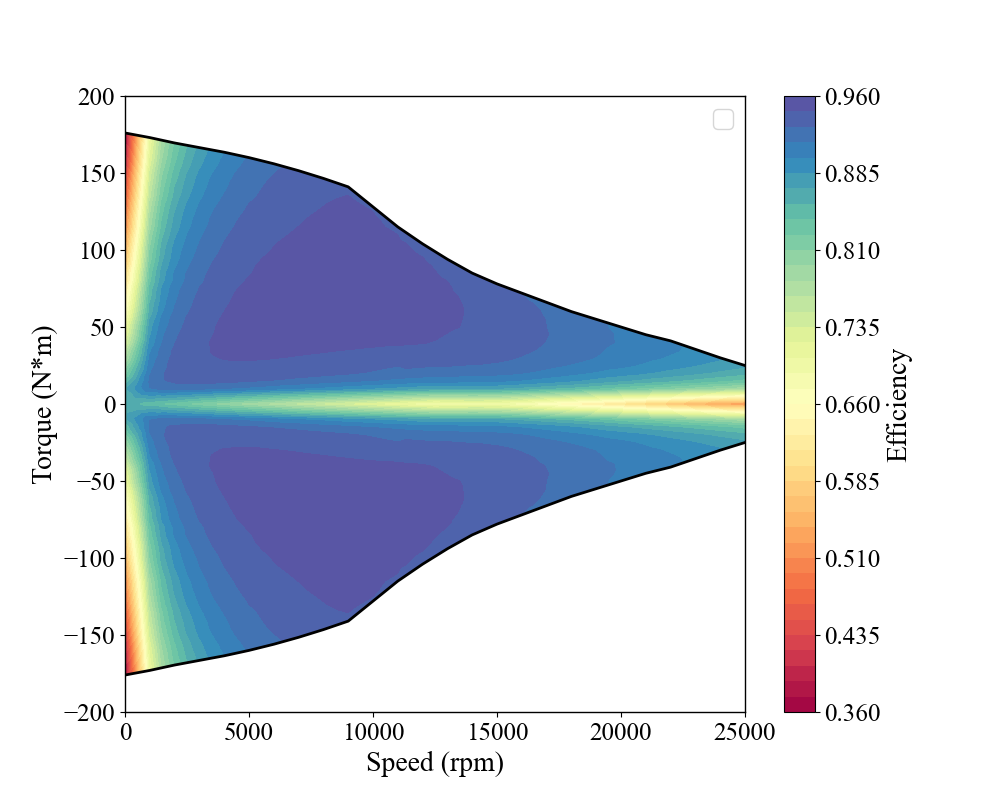}}
\caption{Efficiency map of the electric motor.}
\label{appen2:fig_motor_map}
\vspace{-10pt}
\end{figure}

\begin{figure}[!ht]
\centerline{\includegraphics[width=1.0\columnwidth]{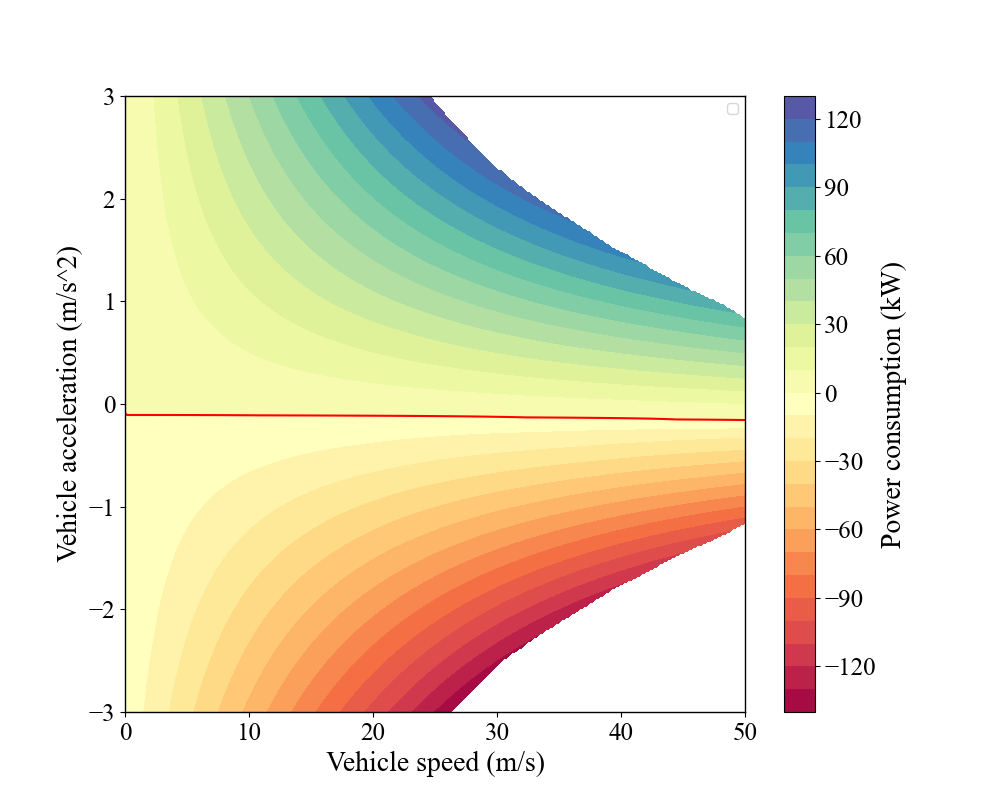}}
\caption{Contour plot of the fitted energy consumption model with respect to vehicle velocity and acceleration.}
\label{appen3:fig_power_distribution}
\vspace{-10pt}
\end{figure}

\begin{figure}[!ht]
\centerline{\includegraphics[width=1.0\columnwidth]{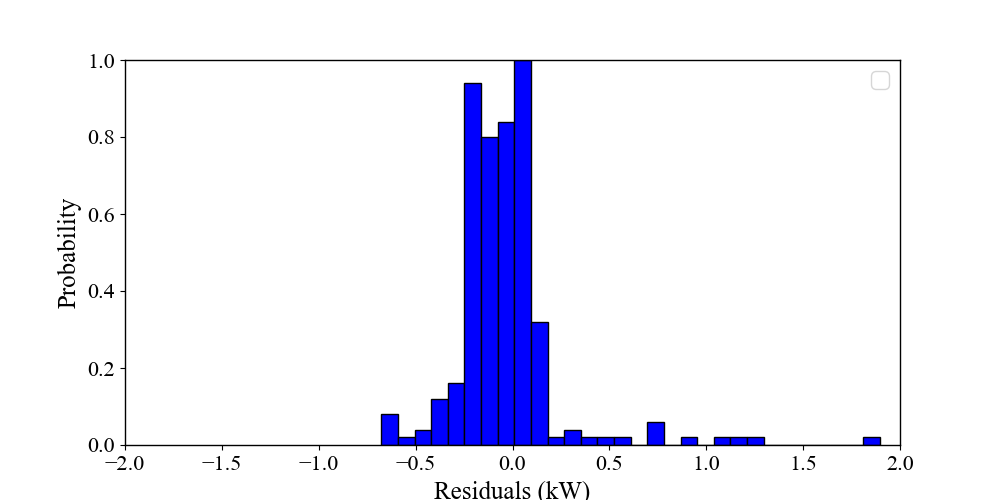}}
\caption{Distribution of the fitting residuals.}
\label{appen4:fig_residul_power}
\vspace{-10pt}
\end{figure}

\subsubsection{\textbf{Vehicle Behavior Modeling}}
The behaviors of vehicles within CACC are effectively modeled using the optimal velocity model (OVM) \cite{bando1995dynamical}, since it accurately reflects the driving behaviors of humans \cite{chu2020multiagent}. Therefore, the formulation for the behavior of the $i$th vehicle is defined as follows:
\begin{equation}
\begin{gathered}
       u_{i}=\alpha_{i}\left(v^{\circ}\left(d_{i} ; d^{s}, d^{g}\right)-v_{i}\right)+\beta_{i}\left(v_{i-1}-v_{i}\right) \\
           v^{\circ}(d_{i}) \triangleq \begin{cases}0, & \text { if } d_{i}<d^{s}, \\ \frac{1}{2} v_{\max }\left(1-\cos \left(\pi \frac{d_{i}-d^{s}}{d^{g}-d^{s}}\right)\right), & \text { if } d^{s} \leq d_{i} \leq d^{g}, \\ v_{\max }, & \text { if } d_{i}>h^{g}\end{cases}
\end{gathered}
\label{eq8}
\end{equation}
where $\alpha_{i}$ and $\beta_{i}$ are the IVS gain and relative velocity gain, respectively. These coefficients are instrumental in mimicking the decision-making process of human drivers, highlighting how both the IVS and the relative velocity contribute to adjustments in acceleration. Specifically, $d^{s}=5 \mathrm{~m}$ and $d^{g}=35 \mathrm{~m}$ denote the stop IVS and the IVS at full velocity for analyzing the behavior of traffic flow. Additionally, $v^{\circ}$ represents the IVS-based velocity policy. This policy function is continuous and differentiable, which is beneficial for computational models and simulations in the environment of the MARL framework. The smooth transition between different phases of the policy (stopping, accelerating, and cruising at maximum velocity) allows for realistic modeling of vehicle dynamics.

\vspace{-10pt}
\subsection{Comparison with the real-world scenarios from OpenACC}

% \begin{figure}
% \centerline{\includegraphics[width=0.85\columnwidth]{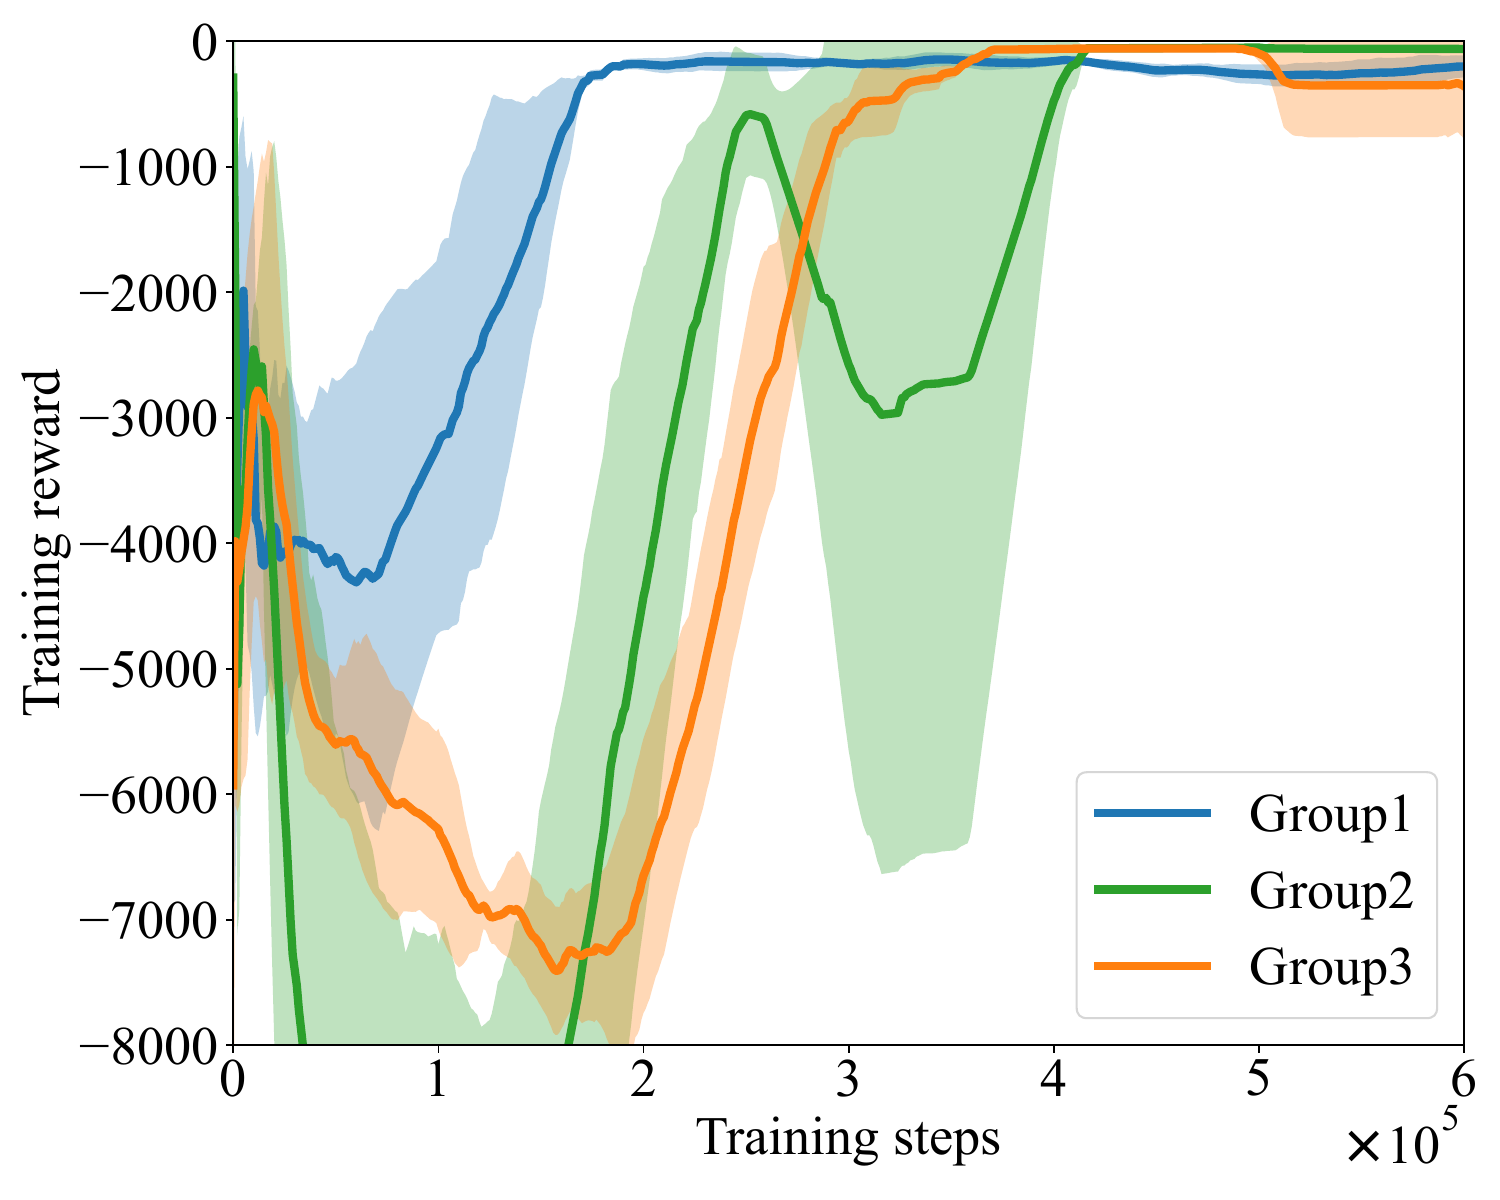}}
% \caption{The comparison with three groups}
% \label{appen5:slow_down}
% \vspace{-10pt}
% \end{figure}

Figure \ref{appen6: cacc_comparison} shows that the learning process of three groups, where Group 1 initially shows a steeper learning curve, potentially indicating quicker adaptation to the set conditions. However, the training process stabilizes at a lower level compared to Groups 2 and 3. This could suggest that tighter spacing introduces complexities in control strategies that are harder to optimize, leading to less optimal performance. Groups 2 and 3 show higher stable rewards, with Group 3 exhibiting the most variance. The variance indicates that while the long spacing allows for potentially better optimization, it can be more susceptible to environmental variations or require more precise control.

\begin{figure}
    \centering
    % Group 1
    \begin{minipage}{0.5\textwidth}
        \centering
            \includegraphics[width=\linewidth]{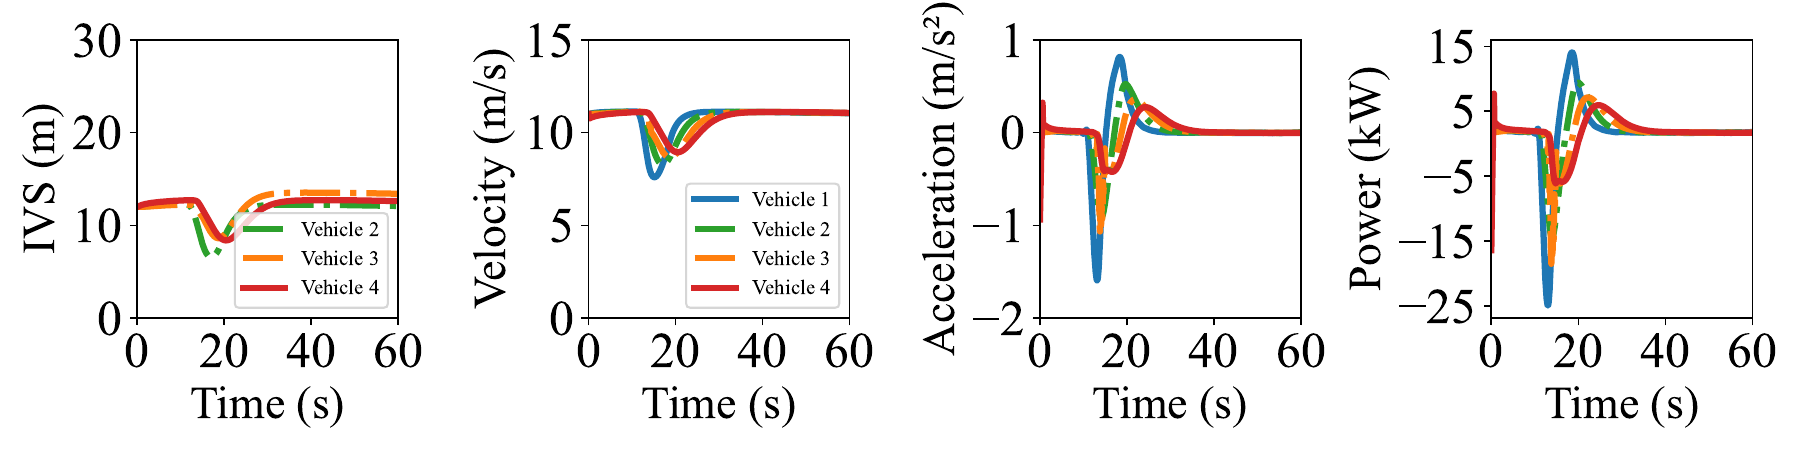}
            \caption*{(a) BDC-MACACC}
    \end{minipage}\hfill
    \begin{minipage}{0.5\textwidth}
        \centering
            \includegraphics[width=\linewidth]{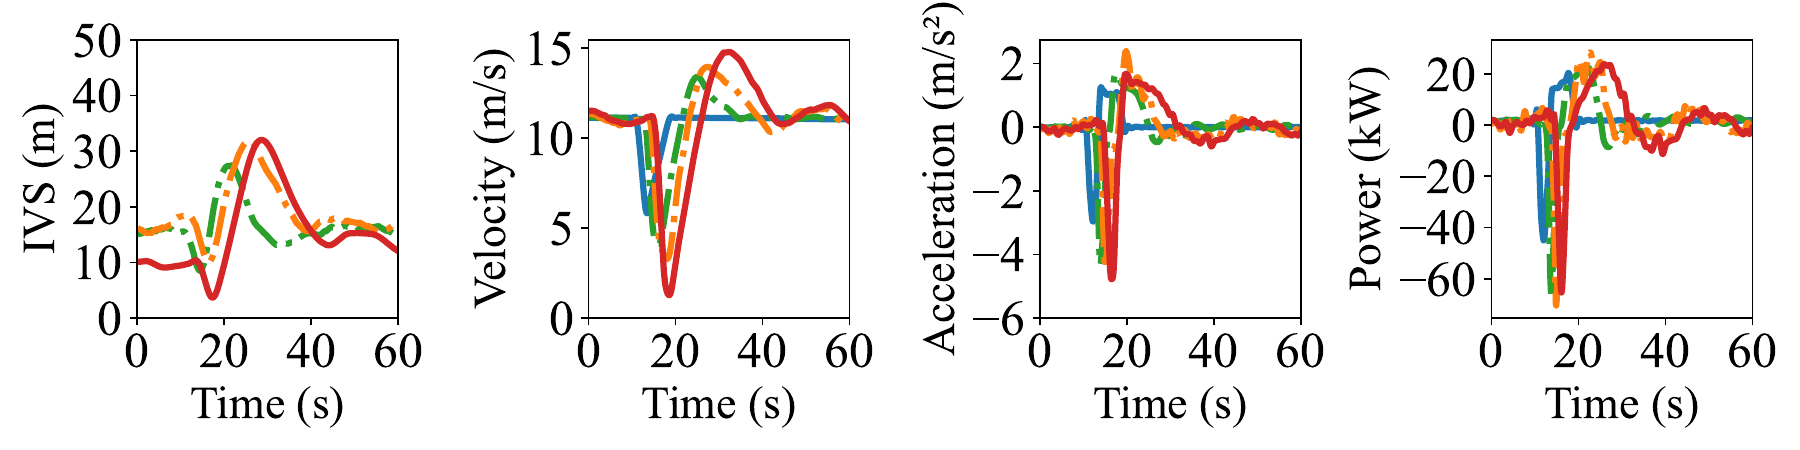}
            \caption*{(b) OpenACC data}
    % \text{(1) Group 1}\\[1ex] 
            
    \end{minipage}
    \vspace{4ex}

     % Group 2
    \begin{minipage}{0.5\textwidth}
        \centering
            \includegraphics[width=\linewidth]{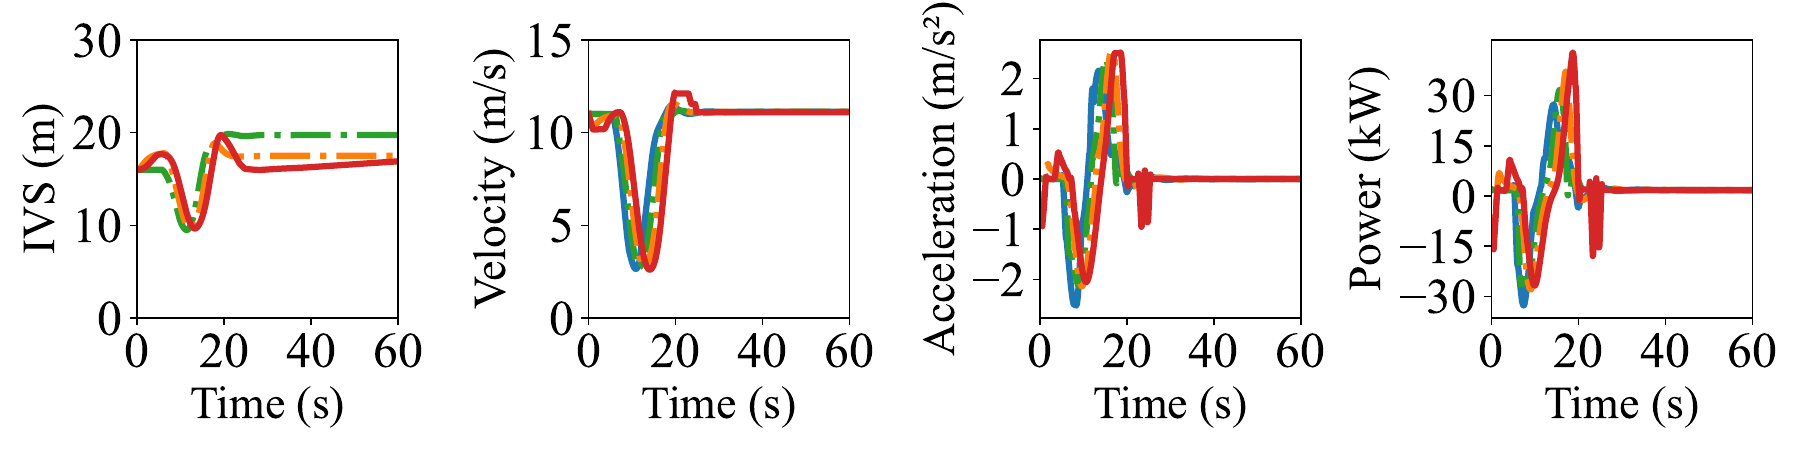}
            \caption*{(a) BDC-MACACC}
    \end{minipage}\hfill
    \begin{minipage}{0.5\textwidth}
        \centering
            \includegraphics[width=\linewidth]{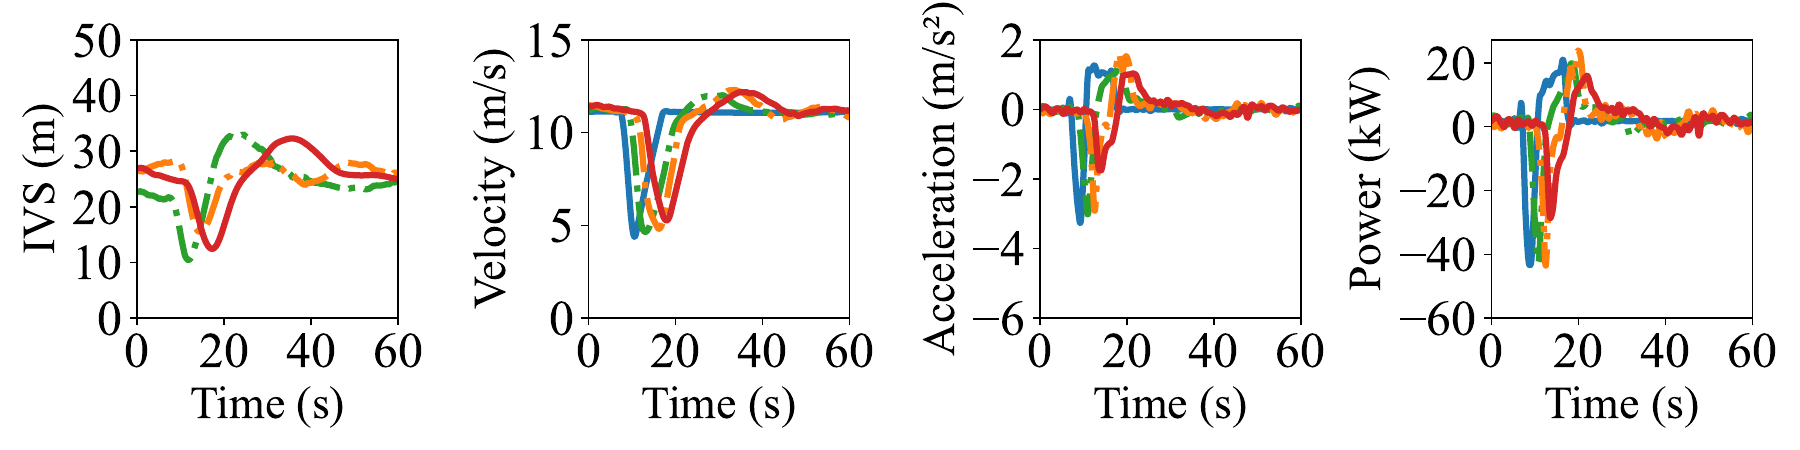}
            \caption*{(b) OpenACC data}
    % \text{(1) Group 2}\\[1ex] 
            
    \end{minipage}
    \vspace{4ex}
    
  % Group 3
    \begin{minipage}{0.5\textwidth}
        \centering
            \includegraphics[width=\linewidth]{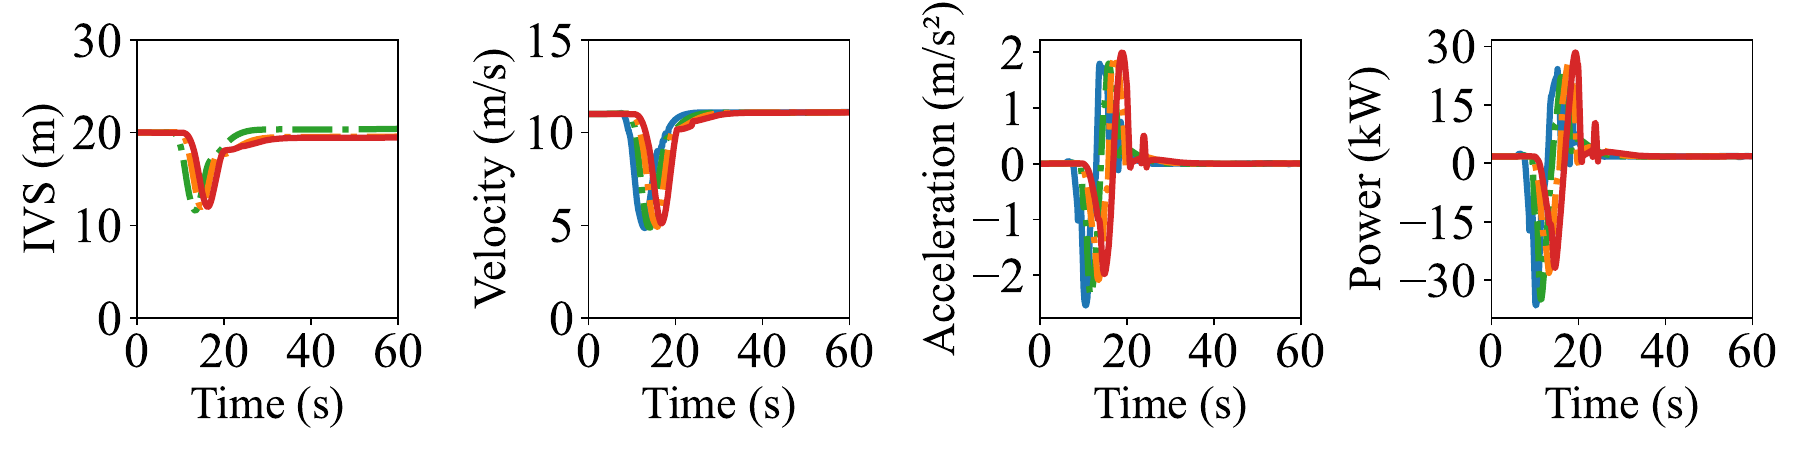}
            \caption*{(a) BDC-MACACC}
    \end{minipage}\hfill
    \begin{minipage}{0.5\textwidth}
        \centering
            \includegraphics[width=\linewidth]{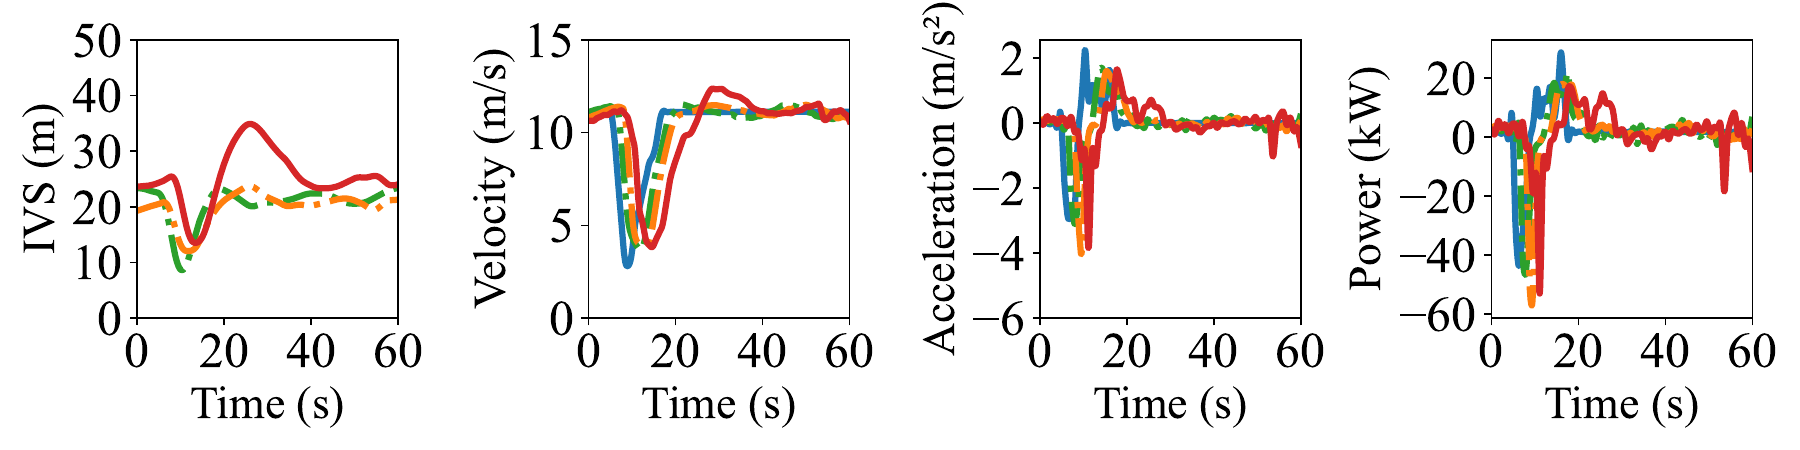}
            \caption*{(b) OpenACC data}
    % \text{(1) Group 3}\\[1ex] 
            
    \end{minipage}
    
    \caption{Comparison of CACC strategies across different groups and corresponding OpenACC data.}
    \label{appen6: cacc_comparison}
\end{figure}
